# Supplementary material for: AI as "Co-founder": GenAI for Entrepreneurship
Source: arXiv:2512.06506 source file (2025-12-06)
Supplement: Supplementary file 1 [file appendix_a1.tex]

&\multicolumn{1}{c}{(1)}&\multicolumn{1}{c}{(2)}&\multicolumn{1}{c}{(3)}\\
               &\multicolumn{1}{c}{Num new firms} & \multicolumn{1}{c}{Num small firms} & \multicolumn{1}{c}{Num large firms} \\  
               % &\multicolumn{1}{c}{\makecell{Number of\\New Firms}} & \multicolumn{1}{c}{\makecell{Number of\\Small\\Businesses}} & \multicolumn{1}{c}{\makecell{Number of\\Large\\Businesses}} \\
\midrule
Post × HighAI  &       18.68\sym{**} &       10.25\sym{***}&       7.278\sym{*}  \\
               &     (7.325)         &     (3.188)         &     (3.872)         \\
[1em]
Constant       &       2.050\sym{**} &       0.842\sym{**} &       1.092\sym{**} \\
               &     (0.811)         &     (0.349)         &     (0.432)         \\
\midrule
Observations   &     2,658,304         &     2,658,304         &     2,658,304         \\
R-squared      &       0.227         &       0.172         &       0.195         \\
City × Quarter FE&         Yes         &         Yes         &         Yes         \\
Prior Count × Calendar Quarter&         Yes         &         Yes         &         Yes         \\
\bottomrule
