# Supplementary material for: AI as "Co-founder": GenAI for Entrepreneurship
Source: arXiv:2512.06506 source file (2025-12-06)
Supplement: Supplementary file 2 [file appendix_a5.tex]

&\multicolumn{4}{c}{Ratio of SE with larger Registered Capital}                         &\multicolumn{4}{c}{Ratio of New Registered Capital to old (Winsorize by quarter)}      \\\cmidrule(lr){2-5}\cmidrule(lr){6-9}
               &\multicolumn{1}{c}{(1)}&\multicolumn{1}{c}{(2)}&\multicolumn{1}{c}{(3)}&\multicolumn{1}{c}{(4)}&\multicolumn{1}{c}{(5)}&\multicolumn{1}{c}{(6)}&\multicolumn{1}{c}{(7)}&\multicolumn{1}{c}{(8)}\\
               &\multicolumn{1}{c}{All firms}&\multicolumn{1}{c}{All firms}&\multicolumn{1}{c}{Small firms}&\multicolumn{1}{c}{Large firms}&\multicolumn{1}{c}{All firms}&\multicolumn{1}{c}{All firms}&\multicolumn{1}{c}{Small firms}&\multicolumn{1}{c}{Large firms}\\
\midrule
Post × HighAI  &    -0.00629\sym{*}  &    -0.00609\sym{*}  &     -0.0542\sym{***}&    -0.00917\sym{***}&      -2.009\sym{***}&      -1.971\sym{***}&      -7.100\sym{***}&      -0.180\sym{***}\\
               &   (0.00320)         &   (0.00316)         &   (0.00483)         &   (0.00241)         &     (0.555)         &     (0.600)         &     (1.148)         &    (0.0230)         \\
[1em]
Constant       &       0.363\sym{***}&       0.363\sym{***}&       0.409\sym{***}&       0.177\sym{***}&       9.531\sym{***}&       8.982\sym{***}&       16.64\sym{***}&       1.200\sym{***}\\
               &  (0.000348)         &  (0.000285)         &  (0.000525)         &  (0.000262)         &    (0.0601)         &    (0.0538)         &     (0.124)         &   (0.00249)         \\
\midrule
Observations   &      375548         &      465081         &      375548         &      375548         &      370690         &      460151         &      370610         &      370861         \\
R-squared      &       0.411         &       0.233         &       0.438         &       0.422         &       0.374         &       0.184         &       0.359         &       0.405         \\
City × Quarter FE&         Yes         &         Yes         &         Yes         &         Yes         &         Yes         &         Yes         &         Yes         &         Yes         \\
Grid × Cal QTR FE&         Yes         &          No         &         Yes         &         Yes         &         Yes         &          No         &         Yes         &         Yes         \\
Grid FE        &          No         &         Yes         &          No         &          No         &          No         &         Yes         &          No         &          No         \\
\bottomrule
