# Supplementary material for: AI as "Co-founder": GenAI for Entrepreneurship
Source: arXiv:2512.06506 source file (2025-12-06)
Supplement: Supplementary file 3 [file appendix_a6.tex]

&\multicolumn{1}{c}{(1)}&\multicolumn{1}{c}{(2)}&\multicolumn{1}{c}{(3)}\\
               &\multicolumn{1}{c}{Num new firms}&\multicolumn{1}{c}{Num small firms}&\multicolumn{1}{c}{Num large firms}\\
\hline
Post × HighAI  &      -1.304         &      -2.038         &       0.666         \\
               &     (1.622)         &     (1.394)         &     (0.600)         \\
[1em]
Constant       &       30.25\sym{***}&       13.28\sym{***}&       15.23\sym{***}\\
               &     (0.135)         &     (0.116)         &    (0.0499)         \\
\hline
Observations   &      977408         &      977408         &      977408         \\
R-squared      &       0.819         &       0.675         &       0.805         \\
City × Quarter FE&         Yes         &         Yes         &         Yes         \\
Grid × Cal QTR FE&         Yes         &         Yes         &         Yes         \\
